# Supplementary material for: Are biofuel mandates cost-effective? -- an analysis of transport fuels and biomass usage to achieve emissions targets in the European energy system
Source: arXiv:2207.03000 source file (2022-07-06)
Supplement: Supplementary file 1 [file Supplementary.pdf]

## Supplementary data

### *S1. Cost assumptions*

Table S1: Overnight investment cost assumptions per technology and year. All costs are given in real 2015 money.

| Technology | Unit | 2020 | 2040 | 2060 | source |
|---|---|---|---|---|---|
| Onshore Wind | €/kW | 1118 | 977 | 963 | [1] |
| Offshore Wind | €/kW | 1748 | 1447 | 1415 | [1] |
| Solar PV (utility-scale) | €/kW | 529 | 329 | 301 | [1] |
| Solar PV (rooftop) | €/kW | 1127 | 661 | 539 | [2] |
| OCGT | €/kW | 453 | 423 | 411 | [1] |
| CCGT | €/kW | 880 | 815 | 800 | [1] |
| Coal power plant | €/kW$_{el}$ | 3845 | 3845 | 3845 | [3] |
| Lignite | €/kW$_{el}$ | 3845 | 3845 | 3845 | [3] |
| Nuclear | €/kW$_{el}$ | 6000 | 6000 | 6000 | [4] |
| Reservoir hydro | €/kW$_{el}$ | 2208 | 2208 | 2208 | [5] |
| Run of river | €/kW$_{el}$ | 3312 | 3312 | 3312 | [5] |
| PHS | €/kW$_{el}$ | 2208 | 2208 | 2208 | [5] |
| Gas CHP | €/kW | 590 | 540 | 520 | [1] |
| Biomass CHP | €/kW$_{el}$ | 3381 | 3061 | 2912 | [1] |
| HVDC overhead | €/MWkm | 400 | 400 | 400 | [6] |
| HVDC inverter pair | €/MW | 150000 | 150000 | 150000 | [6] |
| Battery storage | €/kWh | 232 | 94 | 75 | [1] |
| Battery inverter | €/kW | 270 | 100 | 60 | [1] |
| Home battery storage | €/kWh | 323 | 136 | 108 | [1, 7] |
| Home battery inverter | €/kW | 377 | 144 | 87 | [1, 7] |
| Electrolysis | €/kW$_{el}$ | 650 | 300 | 250 | [1] |
| Fuel cell | €/kW$_{el}$ | 1300 | 950 | 800 | [1] |
| $H_2$ storage underground | €/kWh | 3.0 | 1.5 | 1.2 | [1] |
| $H_2$ storage tank | USD/kWh | 11 | 11 | 11 | [1, 8] |
| direct air capture | €/(t$CO_2$/h) | 7000000 | 5000000 | 4000000 | [1] |
| Methanation | €/kW$_{CH4}$ | 278 | 226 | 226 | [9] |
| Central gas boiler | €/kW$_{th}$ | 60 | 50 | 50 | [1] |
| Domestic gas boiler | €/kW$_{th}$ | 312 | 282 | 268 | [1] |
| Central resistive heater | €/kW$_{th}$ | 70 | 60 | 60 | [1] |
| Domestic resistive heater | €/kWh$_{th}$ | 100 | 100 | 100 | [10] |
| Central water tank storage | €/kWh | 0.6 | 0.5 | 0.5 | [1] |
| Domestic water tank storage | €/kWh | 18 | 18 | 18 | [1, 11] |
| Domestic air-sourced heat pump | €/kW$_{th}$ | 940 | 805 | 760 | [1] |
| Central air-sourced heat pump | €/kW$_{th}$ | 951 | 856 | 856 | [1] |
| Domestic ground-sourced heat pump | €/kW$_{th}$ | 1500 | 1300 | 1200 | [1] |
| $CO_2$ capture in CHP | €/(t$CO_2$/h) | 3300000 | 2400000 | 2000000 | [1] |
| Fischer-Tropsch | €/kW$_{FT}$/a | 2100 | 1100 | 900 | [1] |
| Steam Methane Reforming | €/kW$_{CH4}$ | 540 | 540 | 540 | [12] |
| Steam Methane Reforming with CC | €/kW$_{CH4}$ | 1032 | 1032 | 1032 | [12] |
| BioSNG | €/kW$_{th}$ | 2500 | 1550 | 1500 | [12] |
| BtL | €/kW$_{th}$ | 3850 | 2000 | 2000 | [13, 14] |
| biogas plus hydrogen | €/kW$_{CH4}$ | 907 | 604 | 453 | [1] |
| industrial heat pump medium temperature | €/kW | 871 | 730 | 700 | [1] |
| industrial heat pump high temperature | €/kW | 1045 | 876 | 840 | [1] |
| electric boiler steam | €/kW | 80 | 70 | 70 | [1] |
| gas boiler steam | €/kW | 54 | 45 | 45 | [1] |
| solid biomass boiler steam | €/kW | 618 | 563 | 536 | [1] |
| methanolisation | €/kW$_{MeOH}$ | 4513 | 2256 | 1504 | [1] |

Table S2: Efficiency, lifetime and FOM cost per technology (values shown corresponds to 2020).

| Technology | FOM[a] [%/a] | Lifetime [a] | Efficiency | Source |
|---|---|---|---|---|
| Onshore Wind | 1.3 | 27 | | [1] |
| Offshore Wind | 2.3 | 27 | | [1] |
| Solar PV (utility-scale) | 1.7 | 35 | | [1] |
| Solar PV (rooftop) | 1.2 | 30 | | [2] |
| OCGT | 1.8 | 25 | 0.4 | [1] |
| CCGT | 3.3 | 25 | 0.56 | [1] |
| Coal power plant | 1.6 | 40 | 0.33 | [3] |
| Lignite | 1.6 | 40 | 0.33 | [3] |
| Nuclear | 1.4 | 60 | 0.33 | [3] |
| Reservoir hydro | 1.0 | 80 | 0.9 | [5] |
| Run of river | 2.0 | 80 | 0.9 | [5] |
| PHS | 1.0 | 80 | 0.75 | [5] |
| Gas CHP | 3.3 | 25 | | [1] |
| Biomass CHP | 3.6 | 25 | | [1] |
| HVDC overhead | 2.0 | 40 | | [6] |
| HVDC inverter pair | 2.0 | 40 | | [6] |
| Battery storage | | 20 | | [1] |
| Battery inverter | 0.2 | 10 | 0.95 | [1] |
| Home battery storage | | 20 | | [1, 7] |
| Home battery inverter | 0.2 | 10 | 0.95 | [1, 7] |
| Electrolysis | 2.0 | 25 | 0.66 | [1] |
| Fuel cell | 5.0 | 10 | 0.5 | [1] |
| $H_2$ storage underground | 0.0 | 100 | | [1] |
| $H_2$ storage tank | | 20 | | [1, 8] |
| direct air capture | 5.0 | 20 | | [1] |
| Methanation | 4.0 | 30 | 0.8 | [9] |
| Central gas boiler | 3.2 | 25 | 1.03 | [1] |
| Domestic gas boiler | 6.6 | 20 | 0.97 | [1] |
| Central resistive heater | 1.5 | 20 | 0.99 | [1] |
| Domestic resistive heater | 2.0 | 20 | 0.9 | [10] |
| Central water tank storage | 0.5 | 20 | | [1] |
| Domestic water tank storage | 1.0 | 20 | | [1, 11] |
| Water tank charger/discharger | | | 0.84 | |
| Domestic air-sourced heat pump | 3.0 | 18 | | [1] |
| Central air-sourced heat pump | 0.2 | 25 | 3.4 | [1] |
| Domestic ground-sourced heat pump | 1.9 | 20 | | [1] |
| $CO_2$ capture in CHP | 3.0 | 25 | | [1] |
| Fischer-Tropsch | 3.0 | 25 | 0.65 | [1] |
| Steam Methane Reforming | 5.4 | 25 | 0.74 | [12] |
| Steam Methane Reforming with CC | 5.4 | 25 | 0.67 | [12] |
| BioSNG | 1.6 | 25 | 0.6 | [12] |
| BtL | 2.4 | 25 | 0.45 | [1, 14] |
| biogas plus hydrogen | 4.0 | 25 | | [1] |
| industrial heat pump medium temperature | 0.1 | 20 | 2.55 | [1] |
| industrial heat pump high temperature | 0.1 | 20 | 2.95 | [1] |
| electric boiler steam | 1.3 | 25 | 0.99 | [1] |
| gas boiler steam | 3.7 | 25 | 0.92 | [1] |
| solid biomass boiler steam | 5.5 | 25 | 0.89 | [1] |
| methanolisation | 1.2 | 20 | | [1] |

[a] Fixed Operation and Maintenance (FOM) costs are given as a percentage of the overnight cost per year.
[b] Hydroelectric facilities are not expanded in this model and are considered to be fully amortized.
[c] Coefficient of performance (COP) of heat pumps is modelled as a function of temperature, as described in the text.

Table S3: Costs and emissions coefficient of fuels.

| Fuel | Cost [€/$MWh_{th}$] | Source | Emissions [$tCO_2/MWh_{th}$] | Source |
|---|---|---|---|---|
| coal | 8.2 | [15] | 0.336 | [16] |
| lignite | 2.9 | [5] | 0.407 | [16] |
| gas | 20.1 | [15] | 0.198 | |
| oil | 50.0 | [17] | 0.257 | |
| uranium | 2.6 | [3] | 0 | |

## Supplemental References


[1] Technology Data for Generation of Electricity and District Heating, update November 2019, Tech. rep., Danish Energy Agency and Energinet.dk (2019).
URL https://ens.dk/en/our-services/projections-and-models/technology-data/technology-data-generation-electricity-and

[2] E. Vartiainen, G. Masson, C. Breyer, The true competitiveness of solar PV: a European case study, Tech. rep., European Technology and Innovation Platform for Photovoltaics (ETIP) (2017).
URL http://www.etip-pv.eu/fileadmin/Documents/ETIP_PV_Publications_2017-2018/LCOE_Report_March_2017.pdf

[3] Lazard's Levelized Cost of Energy Analysis, version 13.0.
URL https://www.lazard.com/media/451086/lazards-levelized-cost-of-energy-version-130-vf.pdf

[4] X. Kan, F. Hedenus, L. Reichenberg, The cost of a future low-carbon electricity system without nuclear power – the case of sweden, Energy 195 (2020) 117015. doi:https://doi.org/10.1016/j.energy.2020.117015.
URL https://www.sciencedirect.com/science/article/pii/S0360544220301225

[5] A. Schröeder, F. Kunz, F. Meiss, R. Mendelevitch, C. von Hirschhausen, Current and prospective costs of electricity generation until 2050, Data Documentation, DIW 68. Berlin: Deutsches Institut.
URL https://www.econstor.eu/handle/10419/80348

[6] S. Hagspiel, C. Jägemann, D. Lindenberger, T. Brown, S. Cherevatskiy, E. Tröster, Cost-optimal power system extension under flow-based market coupling, Energy 66 (2014) 654–666. doi:10.1016/j.energy.2014.01.025.
URL http://www.sciencedirect.com/science/article/pii/S0360544214000322

[7] M. Ram, D. Bogdanov, A. Aghahosseini, A. Gulagi, A. S. Oyewo, M. Child, U. Caldera, K. Sadovskaia, J. Farfan, L. S. Barbosa, S. Khalili, C. Breyer, Global energy system based on 100% renewable energy – power, heat, transport and desalination sectors. Study by Lappeenranta University of Technology and Energy Watch Group, Tech. rep. (2019).
URL http://energywatchgroup.org/new-study-global-energy-system-based-100-renewable-energy

[8] C. Budischak, D. Sewell, H. Thomson, L. Mach, D. E. Veron, W. Kempton, Cost-minimized combinations of wind power, solar power and electrochemical storage, powering the grid up to 99.9% of the time, Journal of Power Sources 225 (2013) 60–74. doi:10.1016/j.jpowsour.2012.09.054.
URL http://www.sciencedirect.com/science/article/pii/S0378775312014759

[9] M. Fasihi, D. Bogdanov, C. Breyer, Long-Term Hydrocarbon Trade Options for the Maghreb Region and Europe—Renewable Energy Based Synthetic Fuels for a Net Zero Emissions World, Sustainability 9 (2) (2017) 306. doi:10.3390/su9020306.
URL https://www.mdpi.com/2071-1050/9/2/306

[10] K. Schaber, Integration of Variable Renewable Energies in the European power system: a model-based analysis of transmission grid extensions and energy sector coupling, Ph.D. thesis, TU München (2013).
URL https://d-nb.info/1058680781/34

[11] N. Gerhardt, A. Scholz, F. Sandau, H. H., Interaktion EE-Strom, Wärme und Verkehr. Tech. rep. Fraunhofer IWES.
URL http://www.energiesystemtechnik.iwes.fraunhofer.de/de/projekte/suche/2015/interaktion_strom_waerme_verkehr.html

[12] Hydrogen supply chain: evidence base, Department for Business, Energy & Industrial Strategy, GovUK, Tech. rep. (2018).
URL https://assets.publishing.service.gov.uk/government/uploads/system/uploads/attachment_data/file/760479/H2_supply_chain_evidence_-_publication_version.pdf

[13] D. Thrän, J. Ponitka, O. Arendt, V. Lenz, J. Daniel-Gromke, W. Stinner, A. Ortwein, M. Zeymer, A. Gröngröft, F. Müller-Langer, M. Klemm, J. Braun, W. Zeug, S. O'Keeffe, M. Millinger, Focus on Bioenergy Technologies, DBFZ Deutsches Biomasseforschungszentrum gemeinnützige GmbH, Leipzig, 2015.
URL https://www.energetische-biomassenutzung.de/publikationen/fokusheft

[14] M. Millinger, J. Ponitka, O. Arendt, D. Thrän, Competitiveness of advanced and conventional biofuels: Results from least-cost modelling of biofuel competition in Germany, Energy Policy 107 (2017). doi:10.1016/j.enpol.2017.05.013.

[15] BP Statistical Review of World Energy.
URL https://www.bp.com/content/dam/bp/business-sites/en/global/corporate/pdfs/energy-economics/statistical-review/bp-stats-review-2019-full-report.pdf

[16] Development of the specific carbon dioxide emissions of the German electricity mix in the years 1990 - 2018, German Environment Agency.
URL https://www.umweltbundesamt.de/sites/default/files/medien/1410/publikationen/2019-04-10_cc_10-2019_strommix_2019.pdf

[17] IEA, World Energy Outlook, International Energy Agency, 2017.
